# Supplementary material for: A New Randomized Block-Coordinate Primal-Dual Proximal Algorithm for Distributed Optimization
Source: arXiv:1706.02882 source file (2019-09-30)
Supplement: Supplementary file 1 [file ProofAppendix.tex]

Sometimes it is convenient to defer a proof to the appendix, and \package{clevethm} eases the annoying jumping to and from appendix and theorem statement with hyperreferences.
This is automatized with some handy commands; the procedure is best explained in the example below.

\noindent
\begin{minipage}[t]{.51\linewidth}%
	\vspace*{-5pt}%
\begin{lstlisting}
\section{Results}\label{sec:label}
	\begin{thm}\label{thm:label}
	This theorem has a long proof.
	\begin{proof}
		See \Cref{@({\color{red}\sf proof:)@thm:label}.
	\end{proof}
	\end{thm}
\begin{appendix}
	@({\color{red}\sf\textbackslash proofsection})@{sec:label}
		\begin{@({\color{red}\sf appendixproof)@}{thm:label}
		This is the proof of the theorem.
		\end{@({\color{red}\sf appendixproof)@}
\end{appendix}
\end{lstlisting}
\end{minipage}%
\hfill%
\begin{minipage}[t]{.48\linewidth}%
	\vspace*{0pt}%
	\standalone[width=\textwidth]{ProofAppendix}
\end{minipage}

\vspace\baselineskip\noindent
Notice that clicking on the hypertexts it is possible to jump back and forth exactly where the proof and the theorem are.
The steps are as follows:
\begin{enumerate}
	\item
		the proof in the appendix will be contained in the environment {\color{red}\tt appendixproof} with the theorem's label as argument;
	\item
		the label of the proof in the appendix will automatically be the same as that of the theorem with `{\color{red}\tt proof:}' prepended;
	\item
		optionally, a dedicated proof section can be started with the command \command{appendixsection} which takes as argument the label of the section whose theorems will be proven.
\end{enumerate}
