# Supplementary material for: A New Randomized Block-Coordinate Primal-Dual Proximal Algorithm for Distributed Optimization
Source: arXiv:1706.02882 source file (2019-09-30)
Supplement: Supplementary file 2 [file additional_Commands.tex]

%\usepackage{mathbbol}  % for mathbb of digits changes regular one though
%\usepackage{algpseudocode}% http://ctan.org/pkg/algorithmicx

%\usepackage{dsfont} % for mathbb of numbers 

\newcommand\mathtight{%														% Tightens math equation
	\thinmuskip=1mu%	Unary operator-arg	sin·x   Default: 3mu
	\medmuskip=2mu%		Binary operator-LR	x·+·y   Default: 4mu
	\thickmuskip=4mu%	Relations-LR		x·=·y   Default: 5mu plus 5mu
	\renewcommand\quad{\hspace*{0.5em}}
	\renewcommand\qquad{\quad\quad}
}%

%\usetikzlibrary{pgfplots.groupplots,matrix}
%\usetikzlibrary{external}


% commands 
\newcommand{\bld}[1]{\boldsymbol{#1}}

\newcommand{\lb}[1]{ {\underline {#1}}} %lower bounds
\newcommand{\ub}[1]{ {\overline {#1}}} %upper bounds
\newcommand{\stsum}[1]{\displaystyle\sum\limits #1} % nice sum
\newcommand{\pte}[1]{ ~\mbox{\color{red} #1}} % pano's comments in equations
\newcommand{\pt}[1]{{\color{red} #1}} % pano's comments
\newcommand{\smallmat}[1]{\left[ \begin{smallmatrix}#1 \end{smallmatrix} \right]}
\newcommand{\eqdef}{\triangleq}
\newcommand{\cprod}{\ell_{\mathrm{prod}}}


\newcommand{\ri}{\mathop{\rm ri}\nolimits}

\newcommand{\cone}{\mathop{\rm cone}\nolimits}
\newcommand{\rint}{\mathop{\rm rint}\nolimits}
\newcommand{\lev}{\mathop{\rm lev}\nolimits}
\newcommand{\aff}{\mathop{\rm aff}\nolimits}
\newcommand{\supp}{\mathop{\rm supp}\nolimits}
\newcommand{\Int}{\mathop{\rm int}\nolimits}
\newcommand{\id}{\mathop{\rm Id}\nolimits}


\newcommand{\blkdiag}{\mathop{\rm blkdiag}\nolimits}
\newcommand{\df}{\mathrm{d}f}
\newcommand{\ddf}{\mathrm{d}^2f}


\newcommand{\ddiag}{\mathop{\rm diag}\nolimits}
\newcommand{\sign}{\mathop{\rm sign}\nolimits}
\newcommand{\soft}{\mathop{\rm soft}\nolimits}
\newcommand{\lmigeq}{\succcurlyeq}


% Sets
\renewcommand{\Re}{{\rm{I\!R}} }

\newcommand{\Nn}{{\rm{I\!N}}}
\newcommand{\Bb}{{\rm I\!B} }
% Hilbert spaces
\newcommand{\ZZ}{\mathcal Z}
\newcommand{\HH}{\mathcal H}
\newcommand{\GG}{\mathcal G}
\newcommand{\KK}{\mathcal K}
\newcommand{\YY}{\mathcal Y}
\newcommand{\XX}{\mathcal X}
% set-valued mappings
\newcommand{\rra}{\rightrightarrows}


\newcommand{\sol}{\mathop{\rm SOL}\nolimits}

\newcommand{\gra}{\mathop{\rm gra}\nolimits}

%\newcommand{\argmin}{\mathop{\rm arg\ min}\nolimits}
%\DeclareMathOperator*{\argmin}{arg\,min}
\DeclareMathOperator*{\argmin}{\arg\!\min}
%\newcommand{\argmin}{\operatornamewithlimits{argmin}}
\newcommand{\stt}{\rm subject\ to}

\newcommand{\ie}{\emph{i.e.}}

\DeclareMathOperator*{\E}{\mathbb{E}}

%\newcommand{\onebb}{{\sf 1\hspace{-2.5pt}I}}
%\newcommand{\onebb}{{\rm 1\hspace{-3.5pt}1}}
\DeclareSymbolFont{bbold}{U}{bbold}{m}{n}
\DeclareSymbolFontAlphabet{\mathbbold}{bbold}

%\newcommand{\bld}[1]{\boldsymbol{#1}}

\tikzstyle{every picture}+=[remember picture]
\tikzstyle{na} = [baseline=-.5ex]
\tikzstyle{every picture}+=[remember picture]
\tikzstyle{na} = [baseline=-.5ex]


\newcommand\Rect[1]{	\tikz[baseline=(char.base)]\node[rectangle,draw , cyan,rounded corners,inner sep=2pt] (char) {#1};}

\newcommand\Rectr[1]{	\tikz[baseline=(char.base)]\node[rectangle,draw , black!30!orange,rounded corners,inner sep=2pt] (char) {#1};}

\newcommand\Rectg[1]{	\tikz[baseline=(char.base)]\node[rectangle,draw , black!30!green,rounded corners,inner sep=2pt] (char) {#1};}



% this is necessary for using background enviroment of pgfplot
\pgfdeclarelayer{background}
\pgfsetlayers{background,main}

%Nick's
%\newcommand{\N}{\mathcal{N}}
\newcommand{\Ne}{\mathcal{N}}
\newcommand{\D}{\mathcal{D}}
\newcommand{\Nin}{\mathcal{N}^{\text{in}}}
\newcommand{\Nout}{\mathcal{N}^{\text{out}}}

\newcommand{\x}{\mathsf{x}}
\newcommand{\y}{\mathsf{y}}
\newcommand{\w}{\mathsf{w}}

\newcommand{\f}{\mathsf{f}}
\newcommand{\g}{\mathsf{g}}
\newcommand{\h}{\mathsf{h}}



%\renewcommand{\S}{\mathcal{S}}
\newcommand{\F}{\mathcal{F}}

\newcommand{\hide}[1]{}
%\newcommand{\done}{\centerline{\textbf{\color{blue} **DONE UP TO HERE**}}}
\definecolor{mygreen}{rgb}{0.0, 0.5, 0.0}
\def\nf#1{{\color{red}#1}}
%\def\nf#1{#1}
\def\nfc#1{\textbf{{\color{purple}NF: #1}}}

\newcommand{\done}{\centerline{\textbf{\color{mygreen} **NF: EDITED UP TO HERE**}}}

\def\pp#1{{\color{red}#1}}
