# Supplementary material for: A New Randomized Block-Coordinate Primal-Dual Proximal Algorithm for Distributed Optimization
Source: arXiv:1706.02882 source file (2019-09-30)
Supplement: Supplementary file 3 [file Proofs_Theorems__copy_.tex]

\begin{appendixproof}{lem:Fejerlike-dg} 
	We have 
	\normalsize 
	{\mathtight
	\begin{align}
	{\mathbb{E}_k}\left[\|z^{k+1}-Z\|_{S}^{2}\right]	=&	{\mathbb{E}_k}\left[\|z^{k}-Z+\tfrac{\lambda}{mp_{i_{k}}}U_{i_{k}}(T(\hat{z}^{k})-\hat{z}^{k})\|_{S}^{2}\right]\nonumber\\
	=&\|z^{k}-Z\|_{S}^{2}	+{\mathbb{E}_k}\left[\tfrac{2\lambda}{mp_{i_{k}}}\langle z^{k}-Z,U_{i_{k}}(T(\hat{z}^{k})-\hat{z}^{k})\rangle_{S} \right.\\&+\left.\tfrac{\lambda^2}{m^2p^2_{i_{k}}}\|U_{i_{k}}(T(\hat{z}^{k})-\hat{z}^{k})\|_{S}^{2}\right]\nonumber\\
	=&	\|z^{k}-Z\|_{S}^{2}+\sum_{i=1}^{m}\tfrac{2\lambda}{m}\langle z^{k}-Z,U_{i}(T(\hat{z}^{k})-\hat{z}^{k})\rangle_{S}\nonumber\\&+\sum_{i=1}^{m}\tfrac{\lambda^2}{m^2p_{i}}\|U_{i}(T(\hat{z}^{k})-\hat{z}^{k})\|_{S}^{2}. \label{eq:-1-dg}
	\end{align}} \normalsize 
	For the inner product in the right hand side above we have
	\begin{align}
	\sum_{i=1}^{m}\lambda\langle z^{k}-Z,U_{i}(T(\hat{z}^{k})-\hat{z}^{k})\rangle_{S}	&=	\sum_{i=1}^{m}\lambda\langle Sz^{k}-SZ,U_{i}(T(\hat{z}^{k})-\hat{z}^{k})\rangle\nonumber\\&=\lambda\langle  Sz^{k}- SZ,T(\hat{z}^{k})-\hat{z}^{k}\rangle % =\langle z^{k}-Z,\bar{z}^n_k-\hat{z}^{k}\rangle_{\lambda S}
	\label{eq:-3-dg}\end{align}
	For the last term in~\eqref{eq:-1-dg} given that $S$ has scalar diagonals and $\sum_{i=1}^{m}U_i=\id$, we have 
		  \begin{align}
		  \sum_{i=1}^{m}\tfrac{\lambda^2}{p_i}\|U_{i}(T(\hat{z}^{k})-\hat{z}^{k})\|_{S}^{2}  %\leq\sum_{i=1}^{m}\gamma_i\|U_{i_{k}}(\bar{z}^n_k-z^k)\|^{2}=
		   = \lambda^2\|T(\hat{z}^{k})-\hat{z}^{k}\|_{ p^{-1}S}^{2}. \label{eq:-2-dg}
		  \end{align}
	Combining~\eqref{eq:-1-dg},~\eqref{eq:-3-dg} and~\eqref{eq:-2-dg} yields 
	\footnotesize
	\begin{align}
	{\mathbb{E}_k}\left[\|z^{k+1}-Z\|_{S}^{2}\right]	=  \|z^{k}-Z\|_{S}^{2}+ \tfrac{2\lambda}{m}\langle z^{k}-Z,T(\hat{z}^{k})-\hat{z}^{k}\rangle_{S} + \tfrac{\lambda^2}{m^2} \|T(\hat{z}^{k})-\hat{z}^{k}\|_{ p^{-1}S}^{2}. \label{eq:fej-1}
	\end{align} \normalsize
	Setting $Z=z^k$ yields~\eqref{eq:-8-t1}. The inner product in~\eqref{eq:fej-1} can be written as 
	\small 
	{\mathtight\begin{align*}
		\langle z^{k}-Z,T(\hat{z}^{k})-\hat{z}^{k}\rangle_{ S} & =\langle\hat{z}^{k}-Z,T(\hat{z}^{k})-\hat{z}^{k}\rangle_{ S}+\sum_{d\in J(k)}\langle z^{d+1}-z^{d},T(\hat{z}^{k})-\hat{z}^{k}\rangle_{S}\\
	& \leq\langle\hat{z}^{k}-Z,T(\hat{z}^{k})-\hat{z}^{k}\rangle_{S}+\tfrac{|J(k)|}{2\epsilon }\|T(\hat{z}^{k})-\hat{z}^{k}\|_{ S}^{2}+\tfrac{\epsilon}{2}\sum_{d\in J(k)}\|z^{d+1}-z^{d}\|_{ S}^{2}
	\end{align*}}\normalsize
	Combining this with~\eqref{eq:fej-1} completes the proof. 
	\end{appendixproof}
	\iffalse 
			\begin{appendixproof}{lem:PDc} 
				Consider 
				$$	P-cD=\left[\begin{array}{cc}
				\Sigma^{-1}(1-c) & (\frac{1}{2}-c)L\\
				(\frac{1}{2}-c)L^{*} & \Lambda^{-1}(1-c)-cL^{*}\Sigma L
				\end{array}\right]. $$
				It is evident that $c<1$ must hold. It follows from Schur complement that $P-cD\succeq 0$ if and only if 
				\begin{equation}
				(1-c)\Lambda^{-1}-cL^{*}\Sigma L - \frac{(\frac{1}{2}-c)^2}{1-c}L^*\Sigma L\succeq 0, 
				\end{equation}
				or equivalently 
				
				\begin{equation}
				4(1-c)^2\Lambda^{-1}-{L^{*}\Sigma L}\succeq 0.
				\end{equation}
				one sufficient condition is to set 
				$$
				c\leq 1- \frac{1}{2}\sqrt{\max^{i=1,\ldots,m}{\tau_i}\sum_{k=1}^{m} \sigma_k\|L_k\|^2}
				$$
			\end{appendixproof}
			\fi 

			
		\begin{appendixproof}{lem:main-dg} 
			It follows from \Cref{lem:Fejerlike-dg} at point $Z=z^\star$ that: 
			\begin{align*}\mathbb{E}_{k}\left[\|z^{k+1}-z^\star\|_{S}^{2}\right]  \leq&\|z^{k}-z^\star\|_{S}^{2}+\tfrac{2\lambda}{m}\langle\hat{z}^{k}-z^\star,T(\hat{z}^{k})-\hat{z}^{k}\rangle_{ S}+\tfrac{\epsilon\lambda}{m}\sum_{d\in J(k)}\|z^{d+1}-z^{d}\|_{ S}^{2}\nonumber\\
			& +\tfrac{\lambda^{2}}{m^{2}}\|T(\hat{{z}}^k)-\hat{z}^{k}\|_{p^{-1}S}^{2}+\tfrac{\lambda|J(k)|}{m\epsilon}\|T(\hat{{z}}^k)-\hat{z}^{k}\|_{ S}^{2},%\label{eq:Fej} 
			\end{align*}
			Using this together with~\Cref{lem:nablaf-dg} % and noting 			\[			\langle\hat{z}^{k}-z^{\star},-\bar{z}_{k}^{n}+\hat{z}^{k}\rangle_{S}	\leq	\tfrac{1}{\lambda_{\min}}\langle\hat{z}^{k}-z^{\star},-\bar{z}_{k}^{n}+\hat{z}^{k}\rangle_{\lambda S},\]
			yields
			\small
			{\mathtight
				\begin{align}
				\langle\nabla \mathsf{f}(x^{\star})-&\nabla \mathsf{f}(x^{k}),x^{\star}  -\bar{x}^{k}\rangle+\|T(\hat{z}^k)-\hat{z}^{k}\|_{\tilde{P}}^{2}\leq\tfrac{m}{2\lambda}\|z^{k}-z^{\star}\|_{S}^{2}-\tfrac{m}{2\lambda}{\mathbb{E}_{k}}\left[\|z^{k+1}-z^{\star}\|_{S}^{2}\right]\nonumber\\
				& +\tfrac{\lambda}{2m}\|T(\hat{z}^k)-\hat{z}^{k}\|_{p^{-1}S}^{2}+\tfrac{|J(k)|}{2\epsilon}\|T(\hat{z}^k)-\hat{z}^{k}\|_{ S}^{2}+\tfrac{\epsilon}{2}\sum_{d\in J(k)}\|z^{d+1}-z^{d}\|_{S}^{2} \label{eq:-13}
				\end{align}} \normalsize
			Next we use the fact that in  $x^{k+1}$ update in \Cref{Alg:asynch}, we have $\hat{x}^k=x^k$ because  as we discussed in \Cref{rem:delay} it involves the self variables. Thus   
			\begin{equation}\label{eq:Ex}
			\mathbb{E}_{k}[x^{k+1}]= x^k+\sum_{i=1}^{m}U_{i,x}(\bar{x}^k-\hat{x}^k)=x^k+\sum_{i=1}^{m}U_{i,x}(\bar{x}^k-{x}^k)=\tfrac{\lambda}{m}\bar{x}^{k}+(1-\tfrac{\lambda}{m}){x}^{k}
			\end{equation} 
			multiply both sides of~~\eqref{eq:-13} by $\tfrac{\lambda}{m}$ and use~\eqref{eq:Ex} to derive
 		\footnotesize 
		 \begin{align*}
		 \mathbb{E}_{k}[\langle\nabla \mathsf{f}(x^{\star})-\nabla \mathsf{f}(x^{k})&,x^{k}-x^{k+1}\rangle]+\tfrac{\lambda}{m}\|T(\hat{z}^k)-\hat{z}^{k}\|_{\tilde{P}}^{2}\leq\tfrac{\lambda}{m}\langle\nabla \mathsf{f}(x^{\star})-\nabla \mathsf{f}(x^{k}),x^{k}-x^{\star}\rangle\\
		 & +\tfrac{1}{2}\|z^{k}-z^{\star}\|_{S}^{2}-\tfrac{1}{2}{\mathbb{E}_{k}}\left[\|z^{k+1}-z^{\star}\|_{S}^{2}\right]+\tfrac{\epsilon\lambda}{2m}\sum_{d\in J(k)}\|z^{d+1}-z^{d}\|_{ S}^{2}\\&+\tfrac{\lambda^{2}}{2m^2}\|T(\hat{z}^k)-\hat{z}^{k}\|_{p^{-1}S}^{2}+\tfrac{\lambda|J(k)|}{2m\epsilon}\|T(\hat{z}^k)-\hat{z}^{k}\|_{ S}^{2}
		 \end{align*}
		\normalsize
			Equivalently
				\footnotesize 
				\begin{align*}\mathbb{E}_{k}[\langle\nabla \mathsf{f}(x^{\star})-\nabla \mathsf{f}(x^{k}) & ,x^{k}-x^{k+1}\rangle]+\tfrac{\lambda}{2m}\|T(\hat{z}^{k})-\hat{z}^{k}\|_{\hat{S}}^{2}\leq\tfrac{\lambda}{m}\langle\nabla \mathsf{f}(x^{\star})-\nabla \mathsf{f}(x^{k}),x^{k}-x^{\star}\rangle\\
				& +\tfrac{1}{2}\|z^{k}-z^{\star}\|_{S}^{2}-\tfrac{1}{2}{\mathbb{E}_{k}}\left[\|z^{k+1}-z^{\star}\|_{S}^{2}\right]+\tfrac{\epsilon\lambda}{2m}\sum_{d\in J(k)}\|z^{d+1}-z^{d}\|_{S}^{2}
				\end{align*}
				\normalsize
			where $$\hat{S}\coloneqq2\tilde{P}-\left(\tfrac{\lambda}{m}p^{-1}+\tfrac{|J(k)|}{\epsilon}\right)S. $$ 
			Next we use coordinate-wise Lipschitz knowing that $x^{k+1}$
			differs from $x^{k}$
			along coordinate $i_{k+1}$	only: 
			\begin{equation}
			\mathsf{f}(x^{k+1})\leq \mathsf{f}(x^{k})+\langle\nabla \mathsf{f}(x^{k}),x^{k+1}-x^{k}\rangle+\frac{\beta_{i_{k}}}{2}\|x^{k+1}-x^{k}\|^{2}
			\end{equation}
			Using this we derive 
			\footnotesize{ \mathtight
		\begin{align*}\mathbb{E}_{k}\left[\mathsf{f}(x^{k+1})-\mathsf{f}(x^{k})-\tfrac{\beta_{i_{k}}}{2}\|x^{k+1}-x^{k}\|^{2}-\langle\nabla \mathsf{f}(x^{\star}),x^{k+1}-x^{k}\rangle\right]+\tfrac{\lambda}{2m}\|T(\hat{z}^{k})-\hat{z}^{k}\|_{\hat{S}}^{2}\leq\\
		+\tfrac{\lambda}{m}\langle\nabla \mathsf{f}(x^{\star})-\nabla \mathsf{f}(x^{k}),x^{k}-x^{\star}\rangle-\tfrac{1}{2}{\mathbb{E}_{k}}\left[\|z^{k+1}-z^{\star}\|_{S}^{2}\right]\\
		+\tfrac{1}{2}\|z^{k}-z^{\star}\|_{S}^{2}+\tfrac{\epsilon\lambda}{2m}\sum_{d\in J(k)}\|z^{d+1}-z^{d}\|_{S}^{2}.
		\end{align*}
		}
			\normalsize 
			From convexity of $\mathsf{f}$, we have  $$\langle\nabla \mathsf{f}(x^{\star})-\nabla \mathsf{f}(x^{k}),x^{k}-x^{\star}\rangle\leq\langle\nabla \mathsf{f}(x^{\star}),x^{k}-x^{\star}\rangle+\mathsf{f}(x^{\star})-\mathsf{f}(x^{k})=-S_{k}^{\star}.$$ This together with definition of $S_k^\star$ yields
			\footnotesize
		\begin{align*}\mathbb{E}_{k}[S_{k+1}^{\star}- & \frac{\beta_{i_{k}}}{2}\|x^{k+1}-x^{k}\|^{2}]+\tfrac{\lambda}{2m}\|T(\hat{z}^{k})-\hat{z}^{k}\|_{\hat{S}}^{2}\leq(1-\frac{\lambda}{m})S_{k}^{\star}\\
		& -\frac{1}{2}\mathbb{E}_{k}\left[\|z^{k+1}-z^{\star}\|_{S}^{2}\right]+\frac{1}{2}\|z^{k}-z^{\star}\|_{S}^{2}+\tfrac{\lambda\epsilon}{2m}\sum_{d\in J(k)}\|z^{d+1}-z^{d}\|_{S}^{2}.
		\end{align*}
			\normalsize 
			Next since 
			 $\mathbb{E}_k\left[\beta_{i_k}\|x^{k+1}-x^k\|^2\right]= \sum_{i=1}^{m}\frac{\beta_i\lambda^2}{m^2p_i}\|(\bar{x}^n_{k})^i-\hat{x}_k^i\|= \frac{\lambda^2}{m^2}\|\bar{x}^n_{k}-\hat{x}_k\|^2_{\beta p^{-1}}$ 
			 \textcolor{red}{again here it is actually $x^k$, this needs to be fixed carefully}
			 
			 a simple rearranging yields: 
		\begin{align*}\mathbb{E}_{k}[S_{k+1}^{\star}+\tfrac{1}{2}\|z^{k+1}-z^{\star}\|_{S}^{2} & ]+\tfrac{\lambda}{2m}\|T(\hat{z}^{k})-\hat{z}^{k}\|_{\hat{S}}^{2}-\tfrac{\lambda^{2}}{2m^{2}}\|\bar{x}_{k}^{n}-\hat{x}_{k}\|_{\beta p^{-1}}^{2}\leq\\
		& (1-\tfrac{\lambda}{m})S_{k}^{\star}+\tfrac{1}{2}\|z^{k}-z^{\star}\|_{S}^{2}+\tfrac{\epsilon\lambda}{2m}\sum_{d\in J(k)}\|z^{d+1}-z^{d}\|_{S}^{2}.
		\end{align*}
		
			Next use~\eqref{eq:xi1} and set $\epsilon=\sqrt{m}$ to derive 
			 	\begin{align*}\mathbb{E}_{k} & \left[S_{k+1}^{\star}+\tfrac{1}{2}\xi_{k+1}(z^{\star})\right]\leq(1-\tfrac{\lambda}{m})S_{k}^{\star}+\tfrac{1}{2}\xi_{k}(z^{\star})\\
			 	& +\tfrac{\lambda}{2m}\left(\tfrac{\tau\lambda}{m\sqrt{m}}\|T(\hat{z}^{k})-\hat{z}^{k}\|_{p^{-1}S}^{2}-\|T(\hat{z}^{k})-\hat{z}^{k}\|_{\hat{S}}^{2}+\tfrac{\lambda}{m}\|\bar{x}_{k}^{n}-\hat{x}_{k}\|_{\beta p^{-1}}^{2}\right)
			 	\end{align*}
			 		noting that the last term is simply $-\tfrac{1}{2m}\|T(\hat{z}^{k})-\hat{z}^{k}\|_{\tilde{S}}^2$ completes the proof. 
			 				
		\end{appendixproof}
